# Supplementary material for: Free Energy and Diffusivity in the Fokker-Planck Theory of Polymer Translocation
Source: arXiv:2512.00407 source file (2025-11-29)
Supplement: Supplementary file 1 [file SM.pdf]

**Supplementary Material for**

**Free Energy and Diffusivity in the Fokker-Planck Theory of Polymer Translocation**

Bhaves R. Sarode and Harshwardhan H. Katkar

(Dated: 28 November 2025)

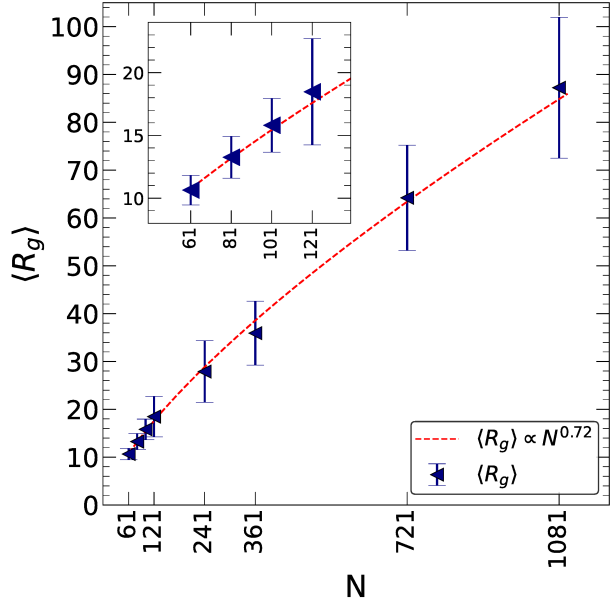

FIG. SI-F1: Variation of  $\langle R_g \rangle$  with the polymer length  $N$ .

## SI1. System Description

The 2000 equilibrium chain conformations were used to calculate radius of gyration  $\langle R_g \rangle$  for a polymer of length  $N$  (Figure SI-F1). The size of the simulation box was chosen to be greater than three times the  $\langle R_g \rangle$  of the respective polymer length and is tabulated in table SI-T1. This ensures that periodic images of the polymer do not interact with its own periodic image.

## SI2. Convergence of Metadynamics Free Energy

We define two representative free energy differences  $\Delta F(t)$  using the instantaneous free energy estimate  $F(x, t)$  at simulation time  $t_{sim}$ . For  $N = 121$ , these are  $\Delta F(t) = (F(x = 20, t) - (F(x = 7, t)))$  and  $\Delta F(t) = (F(x = 120, t) - (F(x = 130, t)))$ . Figure SI-F2 shows both of these  $\Delta F$ 's vs  $t_{sim}$  for one of the five replicas with  $N = 121$  and  $r_p = 1$ . Before the simulation time  $0.15 \times 10^7$  (shown by the red dashed line), each  $\Delta F$  keeps increasing as the slowly added Gaussian bias fills the underlying free energy wells near the two ends of the reaction coordinate (in presence of the added half-harmonic bias potentials). After the dashed line, both  $\Delta F$  values fluctuate around a mean value, suggesting convergence of the

| N    | Box Dimension ( $L_x$ $L_y$ $L_z$ ) |
|------|-------------------------------------|
| 61   | $50 \times 50 \times 80$            |
| 81   | $50 \times 50 \times 80$            |
| 101  | $80 \times 80 \times 80$            |
| 121  | $80 \times 80 \times 100$           |
| 241  | $80 \times 80 \times 120$           |
| 361  | $100 \times 100 \times 150$         |
| 721  | $400 \times 400 \times 750$         |
| 1081 | $600 \times 600 \times 1200$        |

TABLE SI-T1: Simulation box dimensions used for different  $N$ .

metadynamics free energy.

200 estimates of  $F(x,t)$  beyond the dashed line that are  $2.5 \times 10^5$  simulation times apart were collected from each of the five replicas, resulting into 1000 instantaneous estimates for a given choice of  $N$  and  $r_p$ . The time-average and ensemble-average of the shifted instantaneous estimates  $F(x,t) - \min F(x,t)$  is reported as the free energy landscape  $F(x)$  for a given choice of  $N$  and  $r_p$ . The shifting of the instantaneous free energy estimate  $F(x,t)$  is done to remove the arbitrary uniform energy accumulated until time  $t$  shown in Equation (12) of the main text. The average free energy landscapes for  $N$  61, 81, 101, and 121, across  $r_p$  1, 1.4, 1.7, 1.8, 2.1, 3.2, 3.8, and 4, are reported in Figure SI-F4.

### SI3. Fokker-Planck Formalism

The Fokker-Planck equation is solved using the numerical upwinding scheme for the calculation of the spatial gradient, while the temporal dynamics are solved using the MATLAB ode15s function.  $\langle \tau_{\text{FP}} \rangle$  is calculated from the data where  $\int_0^{N+L} W(x,t) dx \geq 10^{-7}$ , after which the change in  $\langle \tau_{\text{FP}} \rangle$  is less than 0.5%.

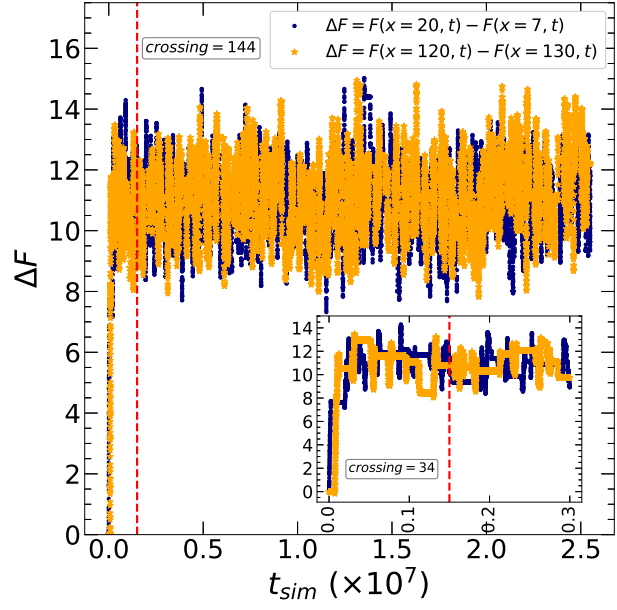

FIG. SI-F2: Metadynamics free energy difference between the threading stage, and pore filling, (shown in blue stars), and the threading stage, and emptying stage (shown in yellow stars) for  $N = 121$  and  $r_p = 1$ .

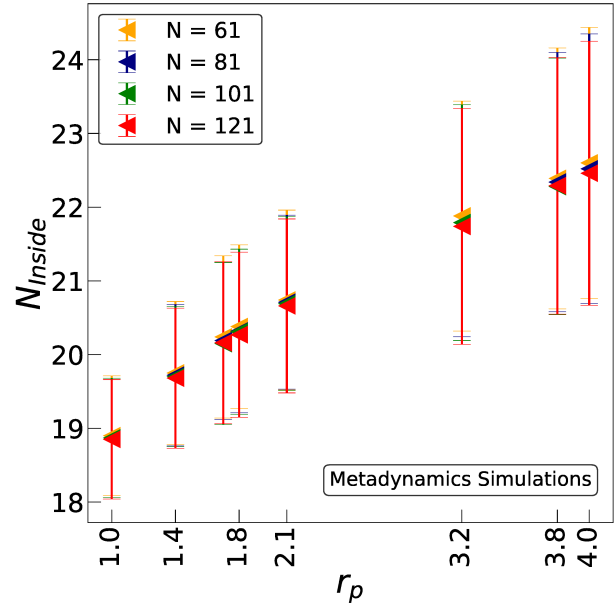

FIG. SI-F3: Average number of beads inside the pore  $N_{\text{inside}}$  during the threading stage calculated from metadynamics simulations.

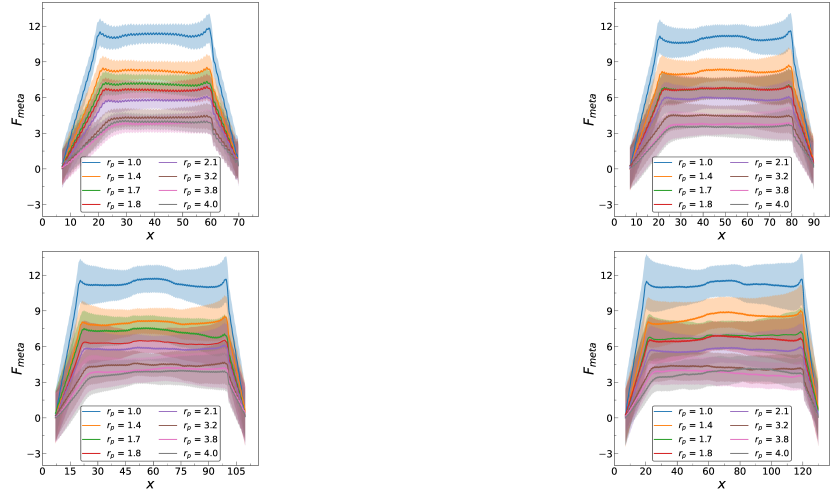

FIG. SI-F4: Free energy landscape generated from metadynamics for  $N=61, 81, 101$ , and  $121$ .

### SI3.1. Theoretical Free Energy

The free energy,  $F(s)$ , corresponding to a translocation state in which  $s(=x)$  segments reside inside the pore and  $N-s$  segments remain in the donor compartment, is expressed as follows:

$$F^{\text{seg}}(s) = s\epsilon_{\text{FP}} \quad (\text{SI-E1a})$$

$$F^{\text{ent}}(s) = s \ln \left( \frac{z}{z_{\text{eff}}} \right) + (1 - \gamma') \ln(N - s) \quad (\text{SI-E1b})$$

$$F^{\text{volt}}(s) = -\frac{|q|Vs^2}{2L} \quad (\text{SI-E1c})$$

where  $z(=6)$  is the coordination number for the cubic lattice model,  $z_{\text{eff}}$  is the effective coordination number,  $\epsilon_{\text{FP}}$  is the per-segment interaction energy inside the pore,  $\gamma'(=0.69)$  is the exponent for the self-avoiding chain,  $q$  is the elementary charge, and  $V$  is the applied transmembrane voltage. For a polymer configuration in which  $m = x - L$  segments have translocated into the recipient compartment and  $N - L - m$  segments remain in the donor compartment, the corresponding free energy,  $F(m)$ , is given by:

$$F^{\text{seg}}(m) = L\epsilon_{\text{FP}} \quad (\text{SI-E2a})$$

$$F^{\text{ent}}(m) = L \ln \left( \frac{z}{z_{\text{eff}}} \right) + (1 - \gamma') \ln[m(N - L - m)] \quad (\text{SI-E2b})$$

$$F^{\text{volt}}(m) = -\frac{|q|VL}{2} + \mu m \quad (\text{SI-E2c})$$

where  $\mu$  is the electrochemical potential. During the final stage of polymer translocation, when the chain is being released from the pore, the free energy,  $F_p$ , corresponding to a configuration with  $N - L + p$  segments in the recipient compartment and  $L - p$  segments remaining inside the pore, where  $p = x - N$  corresponds to the empty length of the pore, is given by:

$$F^{\text{seg}}(p) = (L - p)\epsilon_{\text{FP}} \quad (\text{SI-E3a})$$

$$F^{\text{ent}}(p) = (L - p) \ln \left( \frac{z}{z_{\text{eff}}} \right) + (1 - \gamma') \ln(N - L + p) \quad (\text{SI-E3b})$$

$$F^{\text{volt}}(p) = -\frac{|q|V(L^2 - p^2)}{2L} + \mu(N - L + p) \quad (\text{SI-E3c})$$

The  $\epsilon_{\text{FP}}$  is the difference in per-segment interaction energy between the state when the polymer is outside the nanopore and during the polymer transfer stage.  $\epsilon_{\text{FP}}$  is independent of polymer length  $N$ , as shown in Figure SI-F5. The error bars are shown using a black line. The reported  $\epsilon_{\text{FP}}$  in the manuscript is estimated as the average of pore-polymer averaged interaction energy for  $V = 86.7$  mV.  $z_{\text{eff}}$  is calculated by mapping the theoretical free energy to the metadynamics free energy. The solid left triangles are calculated by using the averaged  $\epsilon_{\text{FP}}$  values for the respective nanopore radius. Whereas the open left triangles are calculated by setting  $\epsilon_{\text{FP}} = 0$ . Our analysis indicates that  $z_{\text{eff}}$  depends solely on the pore radius  $r_p$ , showing no significant dependence on the polymer length( $N$ ), as illustrated in Figure SI-F6. Thus, the reported  $z_{\text{eff}}$  values in the manuscript are averaged over polymer length for the respective nanopore.

Using this formulation, the free energy landscape along with the applied electric field is shown in Figure SI-F8.

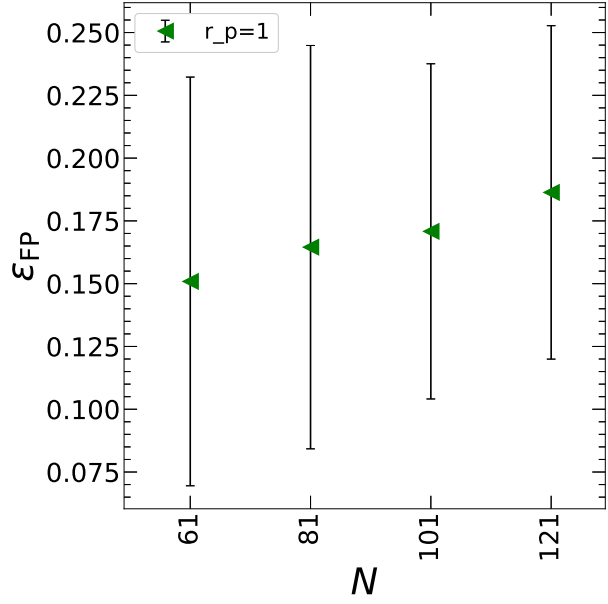

FIG. SI-F5: Independency of  $\epsilon_{FP}$  w.r.t.  $N$

### SI3.2. Numerical Methods

Expanded from equation 17 is discretized using the finite difference scheme.  $x$  is discretised into  $(N + L)/\Delta x$  nodal points where  $\Delta x (= 0.1)$  is the grid spacing in  $x$  shown in the Figure SI-F7.

Spatial derivatives are approximated using the upwinding scheme given in tables SI-T2 – SI-T3. Figure ?? shows sample plots of  $W(x, t)$ .

| <b>i</b>               | <b>Scheme</b>                                                        | <b>Error Order</b> |
|------------------------|----------------------------------------------------------------------|--------------------|
| 1                      | $f'_i = af_i + bf_{i+1} + cf_{i+2}$                                  | $O(\Delta x^2)$    |
| 2                      | $f'_i = df_{i-1} + af_i + bf_{i+1} + cf_{i+2}$                       | $O(\Delta x^3)$    |
| 3                      | $f'_i = ef_{i-2} + df_{i-1} + af_i + bf_{i+1} + cf_{i+2}$            | $O(\Delta x^4)$    |
| $i_{inner}$            | $f'_i = gf_{i-3} + ef_{i-2} + df_{i-1} + af_i + bf_{i+1} + cf_{i+2}$ | $O(\Delta x^4)$    |
| $(N + L)/\Delta x - 2$ | $f'_i = gf_{i-3} + ef_{i-2} + df_{i-1} + af_i + bf_{i+1}$            | $O(\Delta x^4)$    |
| $(N + L)/\Delta x - 1$ | $f'_i = gf_{i-3} + ef_{i-2} + df_{i-1} + af_i$                       | $O(\Delta x^3)$    |

TABLE SI-T2: 1<sup>st</sup> order finite difference schemes and their error orders

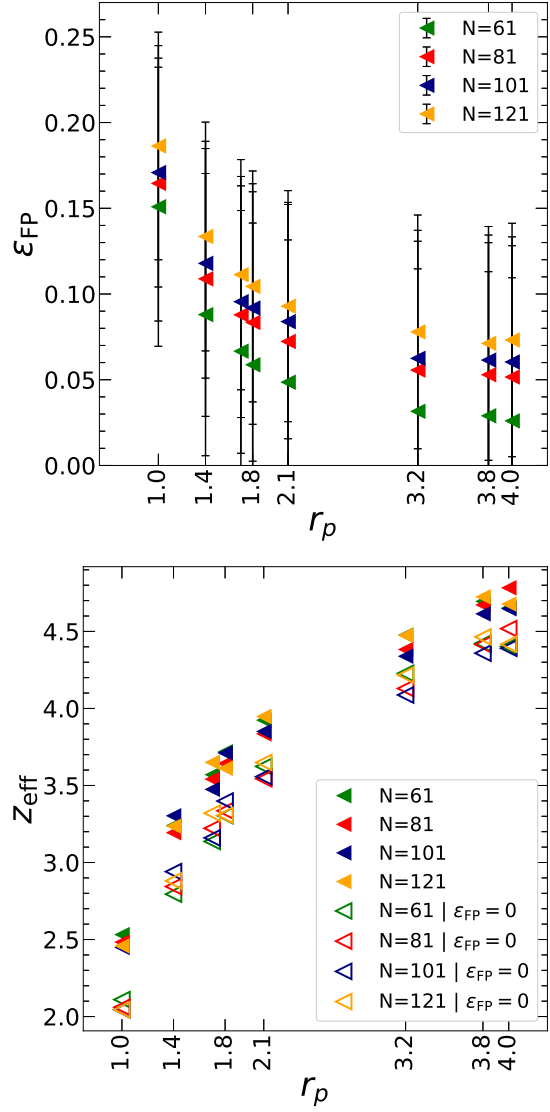

FIG. SI-F6: (a) Dependency of average pore-polymer interaction of polymer inside the nanopore  $\epsilon_{FP}$  on pore radius  $r_p$  for different  $N$ . (b) Variation of the averaged coordination number of polymer beads  $z_{eff}$  inside the nanopore of different  $r_p$  for different  $N$ . The  $z_{eff}$  is adjusted using the averaged values of  $\epsilon_{FP}$  shown in Figure SI-F6 (a) for the respective  $r_p$  shown using the filled left triangle. Whereas the open triangles show the adjusted  $z_{eff}$  by arbitrarily setting  $\epsilon_{FP} = 0$ .

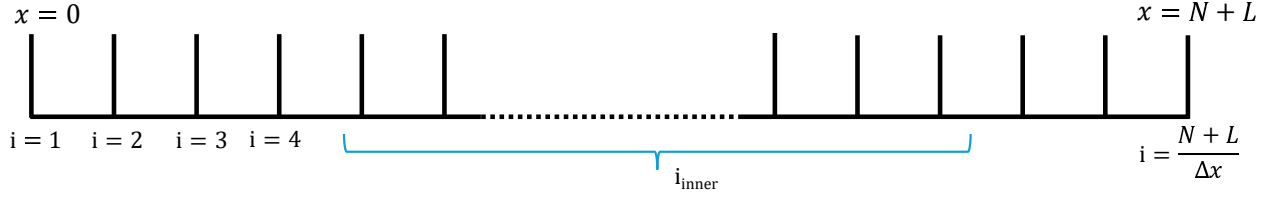

FIG. SI-F7: Discretized grid for numerical upwinding scheme.

| <b>i</b>             | <b>Scheme</b>                                                         | <b>Error Order</b> |
|----------------------|-----------------------------------------------------------------------|--------------------|
| 1                    | $f_i'' = af_i + bf_{i+1} + cf_{i+2}$                                  | $O(\Delta x^1)$    |
| 2                    | $f_i'' = df_{i-1} + af_i + bf_{i+1} + cf_{i+2}$                       | $O(\Delta x^2)$    |
| 3                    | $f_i'' = ef_{i-2} + df_{i-1} + af_i + bf_{i+1} + cf_{i+2}$            | $O(\Delta x^4)$    |
| $i_{inner}$          | $f_i'' = gf_{i-3} + ef_{i-2} + df_{i-1} + af_i + bf_{i+1} + cf_{i+2}$ | $O(\Delta x^4)$    |
| $(N+L)/\Delta x - 2$ | $f_i'' = gf_{i-3} + ef_{i-2} + df_{i-1} + af_i + bf_{i+1}$            | $O(\Delta x^4)$    |
| $(N+L)/\Delta x - 1$ | $f_i'' = gf_{i-3} + ef_{i-2} + df_{i-1} + af_i$                       | $O(\Delta x^2)$    |

TABLE SI-T3:  $2^{nd}$  order finite difference schemes and their error orders

#### SI4. Mean Translocation Time

The probability distribution of the mean translocation time from theoretical and calculated from the Langevin dynamic simulations is in close agreement with each other, as shown in Figure SI-F9. For the calculation of the probability distribution of LD simulations, we have used a log-normal curve to fit the distribution of  $\langle \tau_{LD} \rangle$ .

The probability of successful translocation is independent of polymer length and depends on pore radius and externally applied trans-membrane voltage difference.

The mean translocation time  $\langle \tau_{LD} \rangle$  variation with  $1/V$  is plotted and shown in Figures SI-F11 - SI-F17.

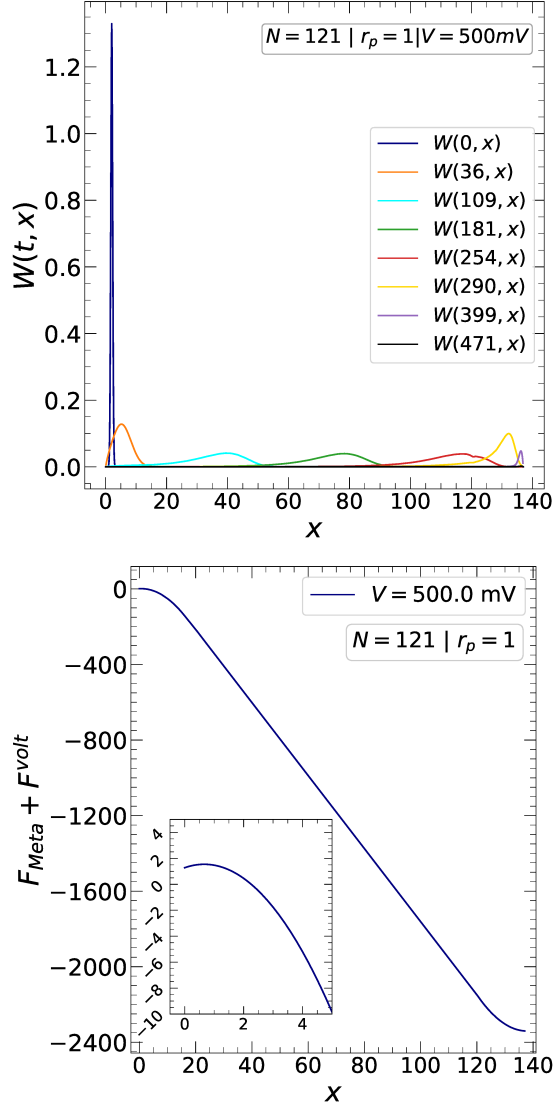

FIG. SI-F8: (a) Probability evolution  $W(x, t)$ . (b) Input free energy from metadynamics with applied externally trans-membrane voltage  $V = 500 \text{ mV}$  for  $N = 121$  and  $r_p = 1$ .

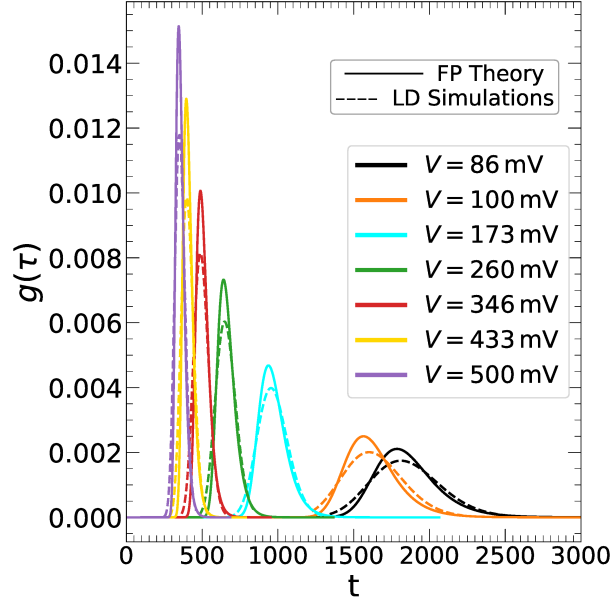

FIG. SI-F9: Probability distribution of mean first passage time  $\langle\tau_{\text{Th}}\rangle$  and mean first passage time  $\langle\tau_{\text{LD}}\rangle$ .

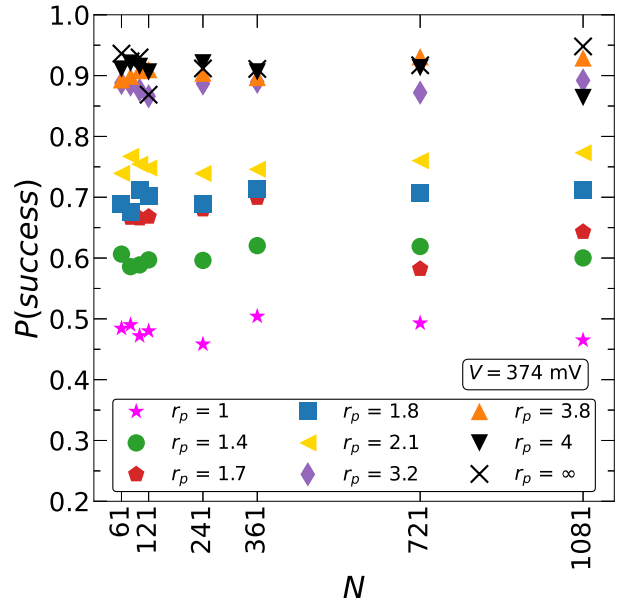

FIG. SI-F10: Variation of probability of successful translocation  $P(\text{success})$  for  $V = 374$  mV.

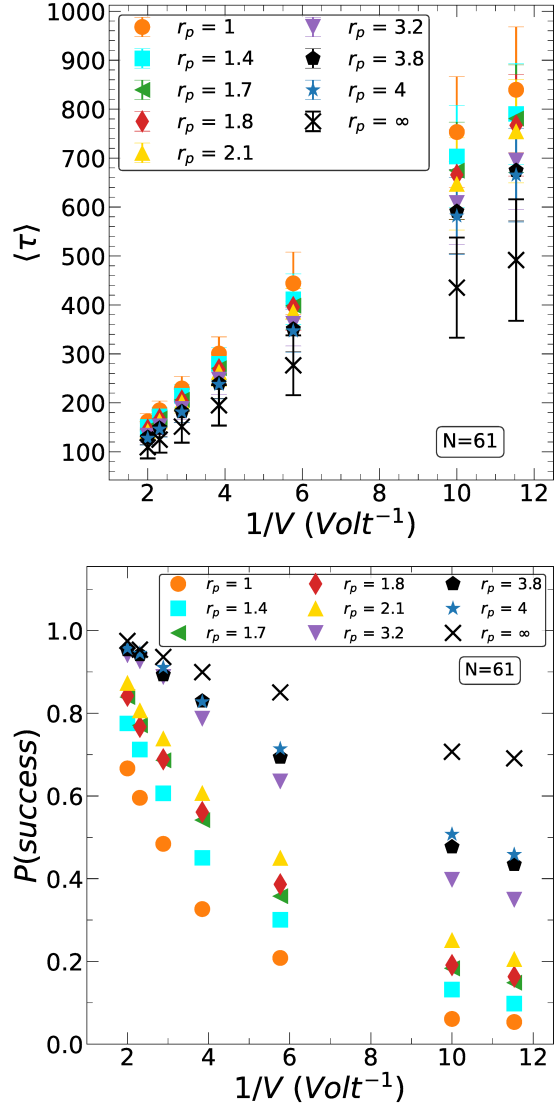

FIG. SI-F11: Linear variation of  $\langle \tau \rangle$  with  $1/V$  the corresponding  $P(\text{success})$  for  $N=61$ .

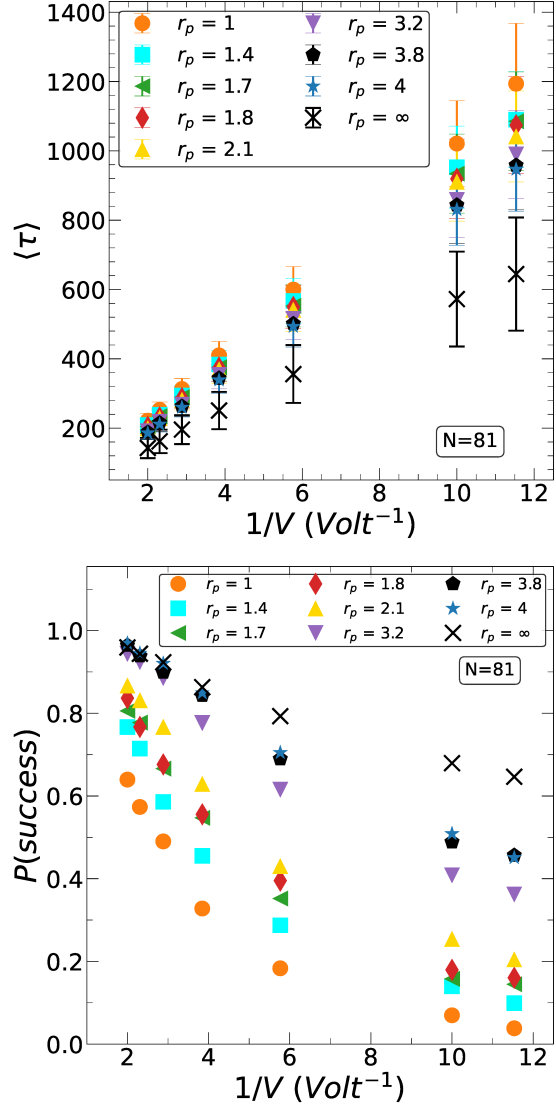

FIG. SI-F12: Linear variation of  $\langle \tau \rangle$  with  $1/V$  the corresponding  $P(\text{success})$  for  $N=81$ .

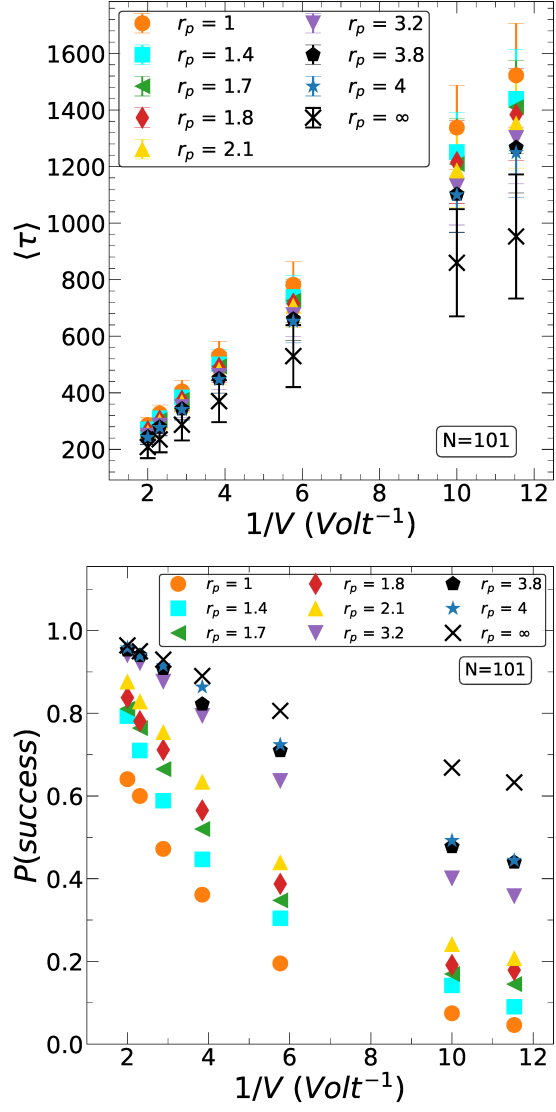

FIG. SI-F13: Linear variation of  $\langle \tau \rangle$  with  $1/V$  the corresponding  $P(\text{success})$  for  $N=101$ .

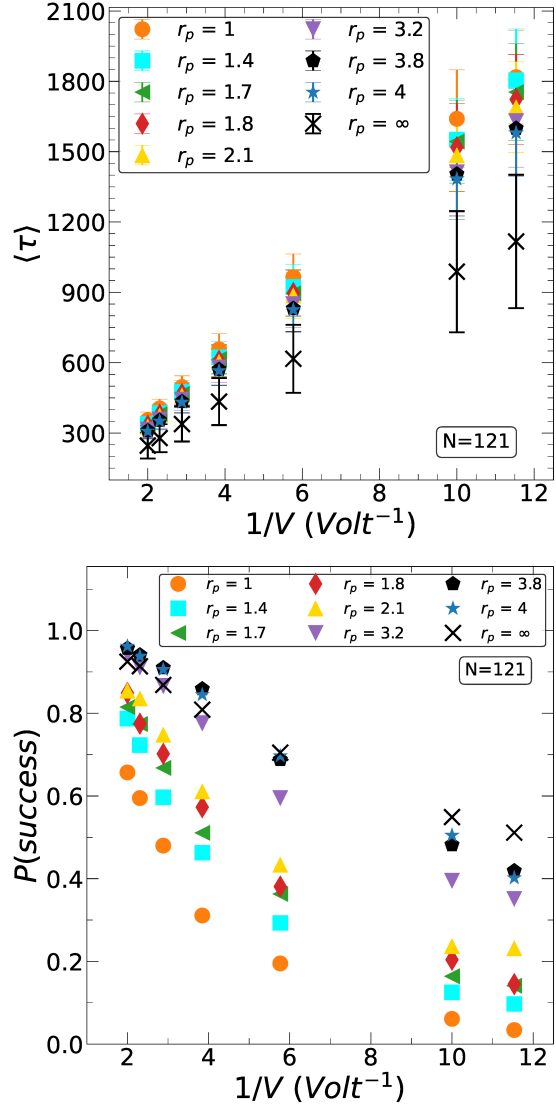

FIG. SI-F14: Linear variation of  $\langle \tau \rangle$  with  $1/V$  the corresponding  $P(\text{success})$  for  $N=121$ .

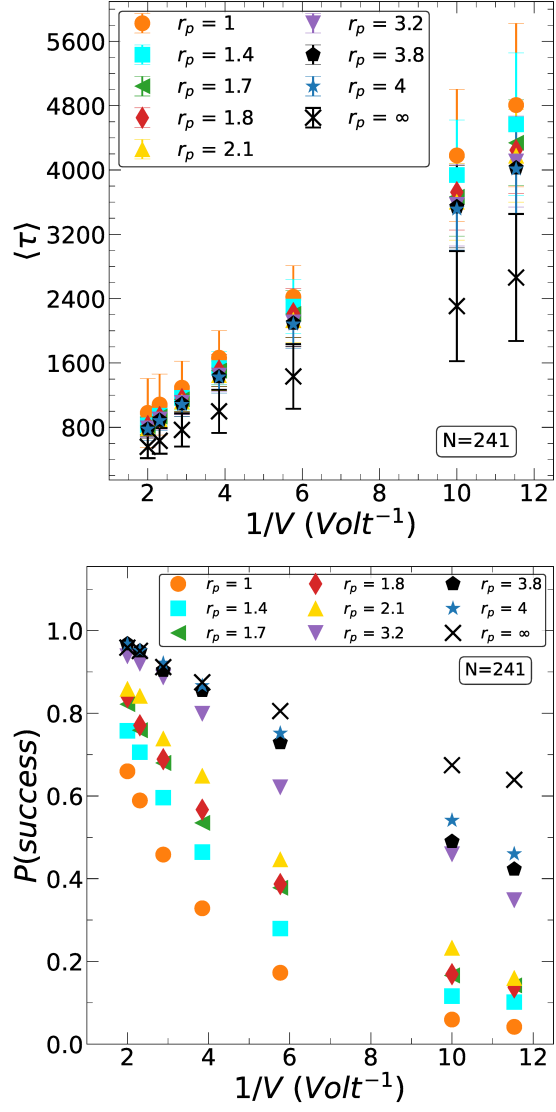

FIG. SI-F15: Linear variation of  $\langle \tau \rangle$  with  $1/V$  the corresponding  $P(\text{success})$  for  $N=241$ .

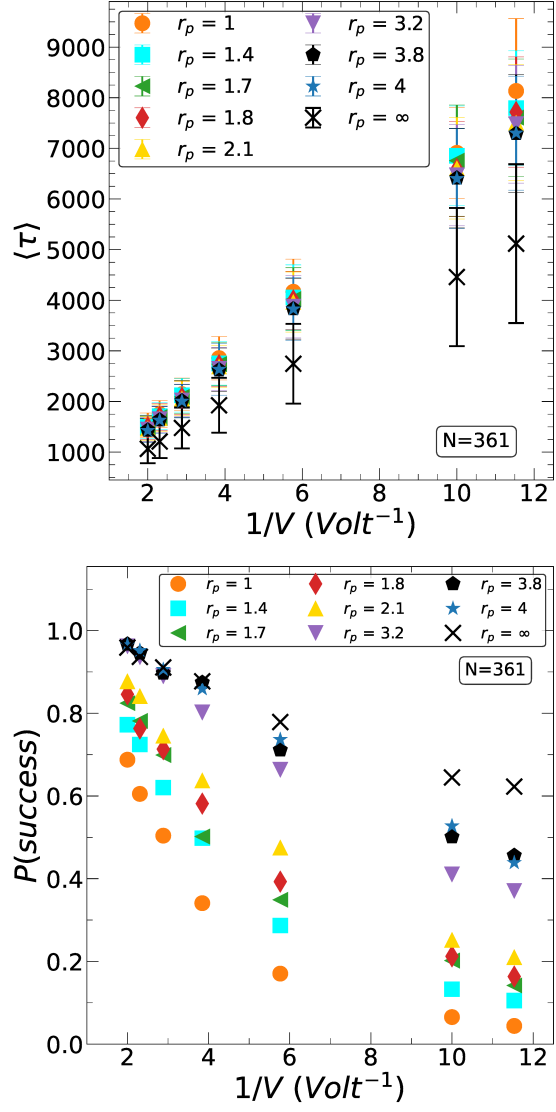

FIG. SI-F16: Linear variation of  $\langle \tau \rangle$  with  $1/V$  the corresponding  $P(\text{success})$  for  $N=361$ .

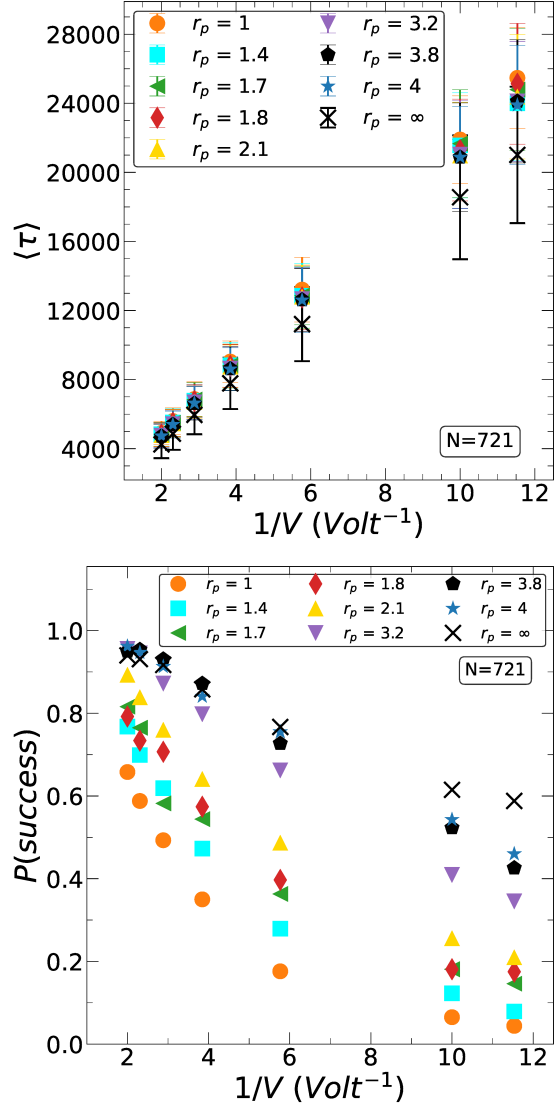

FIG. SI-F17: Linear variation of  $\langle \tau \rangle$  with  $1/V$  the corresponding  $P(\text{success})$  for  $N=721$ .

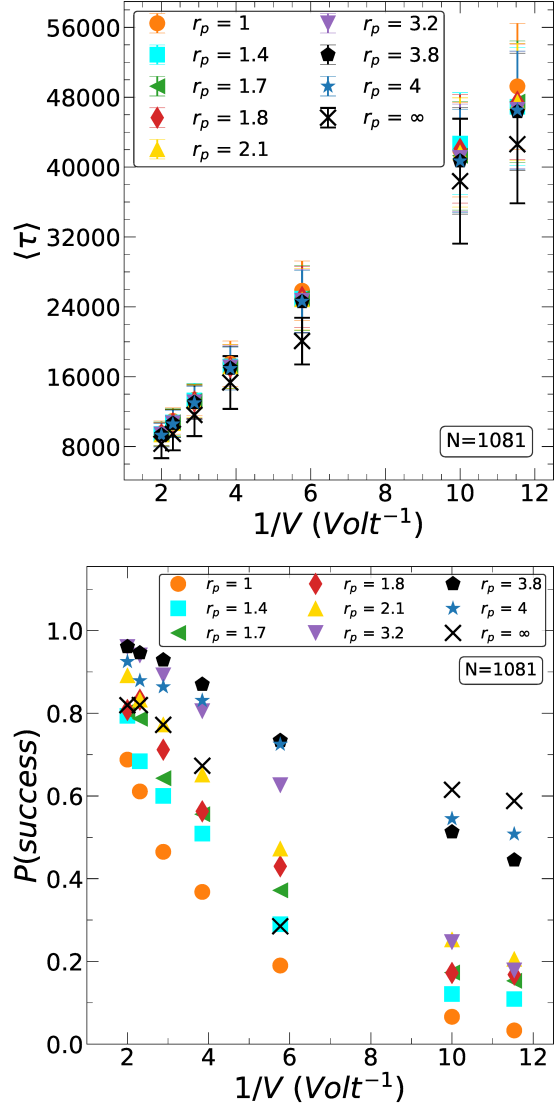

FIG. SI-F18: Linear variation of  $\langle \tau \rangle$  with  $1/V$  the corresponding  $P(\text{success})$  for  $N=1081$ .
